# Supplementary material for: Structured Uncertainty Prediction Networks
Source: arXiv:1802.07079 source file (2018-03-23)
Supplement: Supplementary file 1 [file celeba_denoising.tex]

\def\plotw{0.1\linewidth}

\def\nEig{1000} % Number of eigen vectors

\begin{figure}[btph]
	\centering
	\setlength{\tabcolsep}{1pt} % Reduce spacing between the columns, and add it some to both sides of the vertical bar
	\begin{tabular}{cccc  @{\hspace{5\tabcolsep}}  |  @{\hspace{5\tabcolsep}}  cccc}
	{\small Original } & {\small Input} & {\small DAE} & {\small Ours} & {\small Original } & {\small Input} & {\small DAE} & {\small Ours} \\
	\includegraphics[width=\plotw]{supp_img/celeba/denoising/input/0} &
	\includegraphics[width=\plotw]{supp_img/celeba/denoising/input_noisy/0} &
	\includegraphics[width=\plotw]{supp_img/celeba/denoising/denoising_ae/0} &
	\includegraphics[width=\plotw]{supp_img/celeba/denoising/covar/denoised/\nEig/0} &
	\includegraphics[width=\plotw]{supp_img/celeba/denoising/input/1} &
	\includegraphics[width=\plotw]{supp_img/celeba/denoising/input_noisy/1} &
	\includegraphics[width=\plotw]{supp_img/celeba/denoising/denoising_ae/1} &
	\includegraphics[width=\plotw]{supp_img/celeba/denoising/covar/denoised/\nEig/1} \\
	\includegraphics[width=\plotw]{supp_img/celeba/denoising/input/2} &
	\includegraphics[width=\plotw]{supp_img/celeba/denoising/input_noisy/2} &
	\includegraphics[width=\plotw]{supp_img/celeba/denoising/denoising_ae/2} &
	\includegraphics[width=\plotw]{supp_img/celeba/denoising/covar/denoised/\nEig/2} &
	\includegraphics[width=\plotw]{supp_img/celeba/denoising/input/3} &
	\includegraphics[width=\plotw]{supp_img/celeba/denoising/input_noisy/3} &
	\includegraphics[width=\plotw]{supp_img/celeba/denoising/denoising_ae/3} &
	\includegraphics[width=\plotw]{supp_img/celeba/denoising/covar/denoised/\nEig/3} \\
	\includegraphics[width=\plotw]{supp_img/celeba/denoising/input/4} &
	\includegraphics[width=\plotw]{supp_img/celeba/denoising/input_noisy/4} &
	\includegraphics[width=\plotw]{supp_img/celeba/denoising/denoising_ae/4} &
	\includegraphics[width=\plotw]{supp_img/celeba/denoising/covar/denoised/\nEig/4} &
	\includegraphics[width=\plotw]{supp_img/celeba/denoising/input/5} &
	\includegraphics[width=\plotw]{supp_img/celeba/denoising/input_noisy/5} &
	\includegraphics[width=\plotw]{supp_img/celeba/denoising/denoising_ae/5} &
	\includegraphics[width=\plotw]{supp_img/celeba/denoising/covar/denoised/\nEig/5} \\
	\includegraphics[width=\plotw]{supp_img/celeba/denoising/input/6} &
	\includegraphics[width=\plotw]{supp_img/celeba/denoising/input_noisy/6} &
	\includegraphics[width=\plotw]{supp_img/celeba/denoising/denoising_ae/6} &
	\includegraphics[width=\plotw]{supp_img/celeba/denoising/covar/denoised/\nEig/6} &
	\includegraphics[width=\plotw]{supp_img/celeba/denoising/input/7} &
	\includegraphics[width=\plotw]{supp_img/celeba/denoising/input_noisy/7} &
	\includegraphics[width=\plotw]{supp_img/celeba/denoising/denoising_ae/7} &
	\includegraphics[width=\plotw]{supp_img/celeba/denoising/covar/denoised/\nEig/7} \\
	\includegraphics[width=\plotw]{supp_img/celeba/denoising/input/8} &
	\includegraphics[width=\plotw]{supp_img/celeba/denoising/input_noisy/8} &
	\includegraphics[width=\plotw]{supp_img/celeba/denoising/denoising_ae/8} &
	\includegraphics[width=\plotw]{supp_img/celeba/denoising/covar/denoised/\nEig/8} &
	\includegraphics[width=\plotw]{supp_img/celeba/denoising/input/9} &
	\includegraphics[width=\plotw]{supp_img/celeba/denoising/input_noisy/9} &
	\includegraphics[width=\plotw]{supp_img/celeba/denoising/denoising_ae/9} &
	\includegraphics[width=\plotw]{supp_img/celeba/denoising/covar/denoised/\nEig/9} \\
	\includegraphics[width=\plotw]{supp_img/celeba/denoising/input/10} &
	\includegraphics[width=\plotw]{supp_img/celeba/denoising/input_noisy/10} &
	\includegraphics[width=\plotw]{supp_img/celeba/denoising/denoising_ae/10} &
	\includegraphics[width=\plotw]{supp_img/celeba/denoising/covar/denoised/\nEig/10} &
	\includegraphics[width=\plotw]{supp_img/celeba/denoising/input/11} &
	\includegraphics[width=\plotw]{supp_img/celeba/denoising/input_noisy/11} &
	\includegraphics[width=\plotw]{supp_img/celeba/denoising/denoising_ae/11} &
	\includegraphics[width=\plotw]{supp_img/celeba/denoising/covar/denoised/\nEig/11} \\
	\includegraphics[width=\plotw]{supp_img/celeba/denoising/input/12} &
	\includegraphics[width=\plotw]{supp_img/celeba/denoising/input_noisy/12} &
	\includegraphics[width=\plotw]{supp_img/celeba/denoising/denoising_ae/12} &
	\includegraphics[width=\plotw]{supp_img/celeba/denoising/covar/denoised/\nEig/12} &
	\includegraphics[width=\plotw]{supp_img/celeba/denoising/input/13} &
	\includegraphics[width=\plotw]{supp_img/celeba/denoising/input_noisy/13} &
	\includegraphics[width=\plotw]{supp_img/celeba/denoising/denoising_ae/13} &
	\includegraphics[width=\plotw]{supp_img/celeba/denoising/covar/denoised/\nEig/13} \\
	\includegraphics[width=\plotw]{supp_img/celeba/denoising/input/14} &
	\includegraphics[width=\plotw]{supp_img/celeba/denoising/input_noisy/14} &
	\includegraphics[width=\plotw]{supp_img/celeba/denoising/denoising_ae/14} &
	\includegraphics[width=\plotw]{supp_img/celeba/denoising/covar/denoised/\nEig/14} &
	\includegraphics[width=\plotw]{supp_img/celeba/denoising/input/15} &
	\includegraphics[width=\plotw]{supp_img/celeba/denoising/input_noisy/15} &
	\includegraphics[width=\plotw]{supp_img/celeba/denoising/denoising_ae/15} &
	\includegraphics[width=\plotw]{supp_img/celeba/denoising/covar/denoised/\nEig/15} \\
	\includegraphics[width=\plotw]{supp_img/celeba/denoising/input/16} &
	\includegraphics[width=\plotw]{supp_img/celeba/denoising/input_noisy/16} &
	\includegraphics[width=\plotw]{supp_img/celeba/denoising/denoising_ae/16} &
	\includegraphics[width=\plotw]{supp_img/celeba/denoising/covar/denoised/\nEig/16} &
	\includegraphics[width=\plotw]{supp_img/celeba/denoising/input/17} &
	\includegraphics[width=\plotw]{supp_img/celeba/denoising/input_noisy/17} &
	\includegraphics[width=\plotw]{supp_img/celeba/denoising/denoising_ae/17} &
	\includegraphics[width=\plotw]{supp_img/celeba/denoising/covar/denoised/\nEig/17} \\
	\includegraphics[width=\plotw]{supp_img/celeba/denoising/input/18} &
	\includegraphics[width=\plotw]{supp_img/celeba/denoising/input_noisy/18} &
	\includegraphics[width=\plotw]{supp_img/celeba/denoising/denoising_ae/18} &
	\includegraphics[width=\plotw]{supp_img/celeba/denoising/covar/denoised/\nEig/18} &
	\includegraphics[width=\plotw]{supp_img/celeba/denoising/input/19} &
	\includegraphics[width=\plotw]{supp_img/celeba/denoising/input_noisy/19} &
	\includegraphics[width=\plotw]{supp_img/celeba/denoising/denoising_ae/19} &
	\includegraphics[width=\plotw]{supp_img/celeba/denoising/covar/denoised/\nEig/19} \\
	\includegraphics[width=\plotw]{supp_img/celeba/denoising/input/20} &
	\includegraphics[width=\plotw]{supp_img/celeba/denoising/input_noisy/20} &
	\includegraphics[width=\plotw]{supp_img/celeba/denoising/denoising_ae/20} &
	\includegraphics[width=\plotw]{supp_img/celeba/denoising/covar/denoised/\nEig/20} &
	\includegraphics[width=\plotw]{supp_img/celeba/denoising/input/21} &
	\includegraphics[width=\plotw]{supp_img/celeba/denoising/input_noisy/21} &
	\includegraphics[width=\plotw]{supp_img/celeba/denoising/denoising_ae/21} &
	\includegraphics[width=\plotw]{supp_img/celeba/denoising/covar/denoised/\nEig/21} 
	\end{tabular}
	\caption{ Denoising experiment, left column: original image without noise, second column: image with added noise, third column: denoising autoencoder result, and right column: our result.
	Our model is able to recover fine details with its structure residual prediction.}
	%\label{fig:celeba_denoising}
\end{figure}
