# Supplementary material for: Structured Uncertainty Prediction Networks
Source: arXiv:1802.07079 source file (2018-03-23)
Supplement: Supplementary file 2 [file celeba_denoising_error_table.tex]

\begin{table}[htpb]
\begin{minipage}[b]{0.49\linewidth}
\centering
\includegraphics[width=\linewidth]{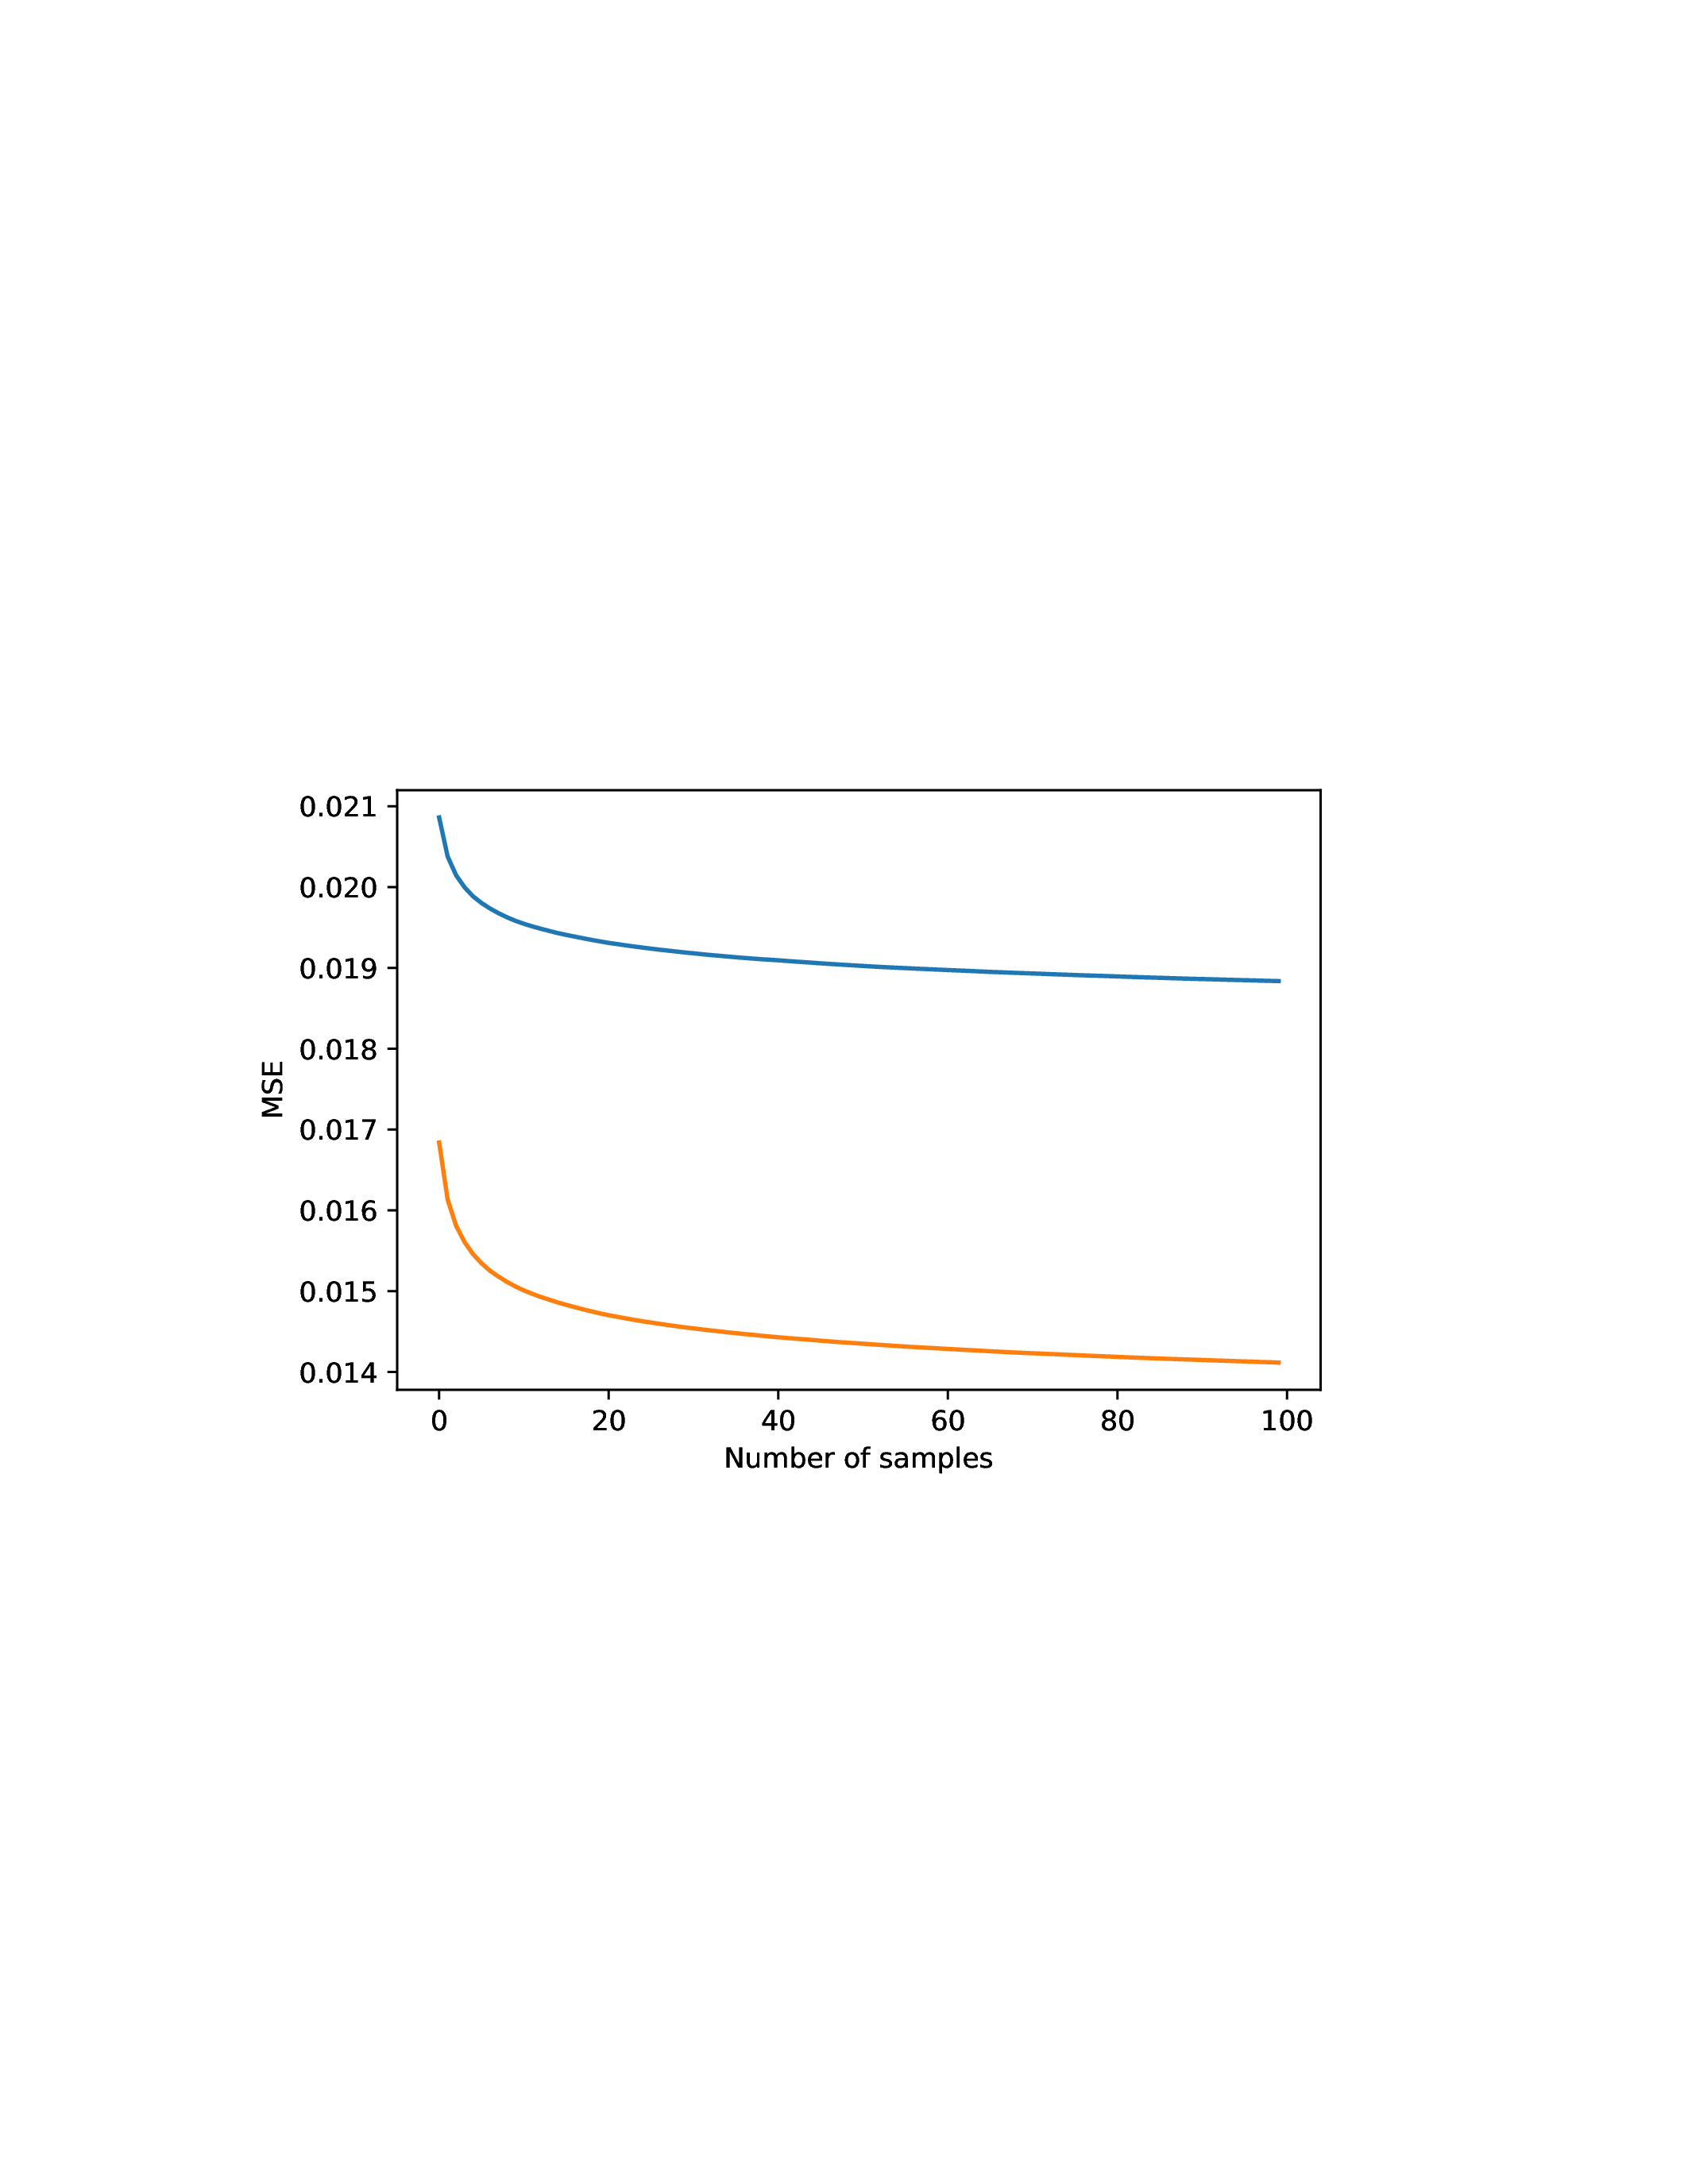}
\captionof{figure}{Quantitative comparison of reconstruction error as the number of samples from $\bSigma$ increases.
On the y-axis is the mean of the MSE (mean squared error) for the best samples and on the x-axis the number of samples taken from $\bSigma$.
Blue denotes a VAE with a diagonal covariance, and orange is used for our structured residual estimation model.
}
\label{fig:plot_error_vs_num_sigma_samples}
\end{minipage}
\end{table}
