# Supplementary material for: Structured Uncertainty Prediction Networks
Source: arXiv:1802.07079 source file (2018-03-23)
Supplement: Supplementary file 3 [file ellipses_error_table.tex]

\begin{minipage}[b]{0.45\linewidth}
\centering\small
\begin{tabularx}{\linewidth}{YY}
	%\toprule
	    & \textbf{NLL} \\ \midrule
	Ground truth & -2.86e2 $\pm$ 2.77 \\ \midrule % Copied from main results in paper
	VAE & -1.34e2 $\pm$ 3.60 \\ \midrule % -133.620361328+-3.60188790921
	Ours-VAE & -1.99e2 $\pm$ 2.91 \\ \midrule % -199.329648844+-2.90913143958
\end{tabularx}
\caption{Quantitative comparison of density estimation error measured as the negative log likelihood (NLL), lower is better.
Our estimation method is able to improve over the VAE simplified noise model.
}
\label{tb:ellipses_error_table}
\end{minipage}
