# Supplementary material for: Structured Uncertainty Prediction Networks
Source: arXiv:1802.07079 source file (2018-03-23)
Supplement: Supplementary file 4 [file ellipses_vae_arch.tex]

\begin{figure}[H]
	\center
	\includegraphics[width=0.6\linewidth]{supp_img/ellipses/vae_arch}
	\caption{VAE architecture for the ellipses dataset.}
	\label{fig:ellipses_vae_arch}
\end{figure}
