# Supplementary material for: Structured Uncertainty Prediction Networks
Source: arXiv:1802.07079 source file (2018-03-23)
Supplement: Supplementary file 5 [file splines_error_table.tex]

\begin{minipage}[b]{0.45\linewidth}
\centering\small
\begin{tabularx}{\linewidth}{YY}
	%\toprule
	    & \textbf{NLL} \\ \midrule
	Ground truth & 18.65 $\pm$ 0.75 \\ \midrule % 18.6538749695+-0.746028781472
	VAE & 36.60 $\pm$ 0.73 \\ \midrule % 36.601210022+-0.733857754571
	Ours-VAE & 19.59 $\pm $ 1.06 \\ \midrule % 19.5856702805+-1.05493193396
\end{tabularx}
\caption{Quantitative comparison of the negative log likelihood (NLL), lower is better.
Our model is able to achieve better results with its more complex uncertainty distribution than a VAE.
}
\label{tb:splines_error_table}
\end{minipage}
