# Supplementary material for: Structured Uncertainty Prediction Networks
Source: arXiv:1802.07079 source file (2018-03-23)
Supplement: Supplementary file 6 [file splines_reconstructions.tex]

\def\plotw{0.49\linewidth}

\def\1img{0}
\def\2img{5}

\begin{figure}[t!]
\setlength{\tabcolsep}{0pt}
\resizebox{\linewidth}{!}{
\begin{tabular}{@{\hspace{3pt}}c @{\hspace{3pt}}c @{\hspace{3pt}}c}
	$n_s$ & &  \\
	1 &
	\includegraphics[align=c, width=\plotw]{img/splines/best_samples/1/\1img} &
	\includegraphics[align=c, width=\plotw]{img/splines/best_samples/1/\2img} \\[24pt]
	10 &
	\includegraphics[align=c, width=\plotw]{img/splines/best_samples/10/\1img} &
	\includegraphics[align=c, width=\plotw]{img/splines/best_samples/10/\2img} \\[24pt]
	100 &
	\includegraphics[align=c, width=\plotw]{img/splines/best_samples/100/\1img} &
	\includegraphics[align=c, width=\plotw]{img/splines/best_samples/100/\2img} \\[24pt]
	\end{tabular}
	}
	\caption{Reconstructions with samples from $\bSigma$, where $n_s$ is the number of samples used.
	The ground-truth spline is depicted in blue, and the estimated one in orange.
	As the number of samples increases the shape of the input is recovered more accurately.}
	\label{fig:spline_reconstructions}
\end{figure}
